# Supplementary material for: HoloFusion: Towards Photo-realistic 3D Generative Modeling
Source: arXiv:2308.14244 source file (2023-08-28)
Supplement: Supplementary file 1 [file suppl_body.tex]

\section{Views2Voxel-grid unprojection mechanism}
\newcommand{\real}{\mathbb{R}}
\newcommand{\bp}{\mathbf{p}}
Given a training video $s$ containing frames $I_j$, we obtain the auxiliary grid $\bar V \in \real^{d \times S \times S \times S}$
of auxiliary features $\bar V_{:mno} \in [-1, 1]^{d}$ by using the following procedure.
The values $m,n,o \in \mathbb{N}$ index the 3D grid of size [$S \times S \times S$].
We first project the 3D coordinate $\bp^{\bar V}_{mno}$ of each grid vertex (corner) $(m,n,o)$  to every video frame $I_j$ and sample corresponding 2D image features.
The 2D image features $f_{mno}^{j}$ are obtained using a frozen ResNet-32 encoder~\cite{he16deep} $E(I_j)$.
We use bilinear interpolation for sampling continuous values and use zero-features for projected points that lie outside the image region on the 3D image plane.
Thus, we obtain $N_\text{frames}$ feature-vectors (corresponding to each frame in the video) for each grid element of the voxel-grid.
We accumulate these features using the accumulator MLP $\mathcal{A}_{acc}$.
The accumulator $\mathcal{A}_{acc}$ takes as input $[f_{mno}^{j}; v^j]$, where $[~;~]$ denotes concatenation and $v^j$ corresponds to the viewing direction of the camera center of $j^{\text{th}}$ frame, and outputs $[\sigma^j_{mno}; {f'}_{mno}^{j}]$.
Here, the value $\sigma^j$ corresponds to a weight for $j^\text{th}$ feature vector and $f'^j$ is an MLP transformed version of the input feature vector.
Lastly, we compute the aggregated feature vector (for each of the voxel grid centers) as a weighted sum of the transformed features:
\begin{equation}
    \bar V_{:mno} = F_{mno} = \sum_{j} \sigma^j_{mno} {f'}_{mno}^{j}.
\end{equation}

% \section{HoloDiffusion anonymous copy}
% An anonymous copy of the CVPR 2023 accepted paper titled \textbf{``HoloDiffusion: Training a 3D diffusion model using 2D Images''} is provided in the supplementary material along with this pdf. Please find the copy enclosed in the zip archive.

\section{\method{Stable-DreamFusion} baseline details}
\paragraph{Implementation  details}  Since no code is available for either of the two 2D diffusion distillation works, DreamFusion \cite{poole2022dreamfusion} and Magic3D \cite{lin2022magic3d}, we resort to using the open-source implementation provided by the GitHub user \href{https://github.com/ashawkey}{ashawkey} titled \href{https://github.com/ashawkey/stable-dreamfusion}{\method{Stable-DreamFusion}} \cite{stable-dreamfusion}. The differences between the implementation and the aforementioned research works are as follows:
\begin{enumerate}
    \item While DreamFusion uses the Imagen \cite{ho2022imagen} diffusion model, and Magic3D uses a combination of Ediff-I \cite{balaji2022ediffi} and StableDiffusion \cite{rombach2021stablediffusion}, the implementation only uses StableDiffusion since Imagen and Ediff-I models are unavilable.

    \item Since the used diffusion network of StableDiffusion performs diffusion in the latent-space, the implementation applies the SDS loss in the latent space and backpropagates the SDS gradients through the perceptual encoder.
    
    \item The DIP generator (backbone) is implemented as a vanilla NeRF \cite{mildenhall20nerf:} as opposed to the Mip-NeRF \cite{barron2021mip} version as used by DreamFusion. 
\end{enumerate}

\paragraph{Prompt builder} 
We use a simple procedure to generate the prompts used for distilling the samples from the \method{Stable-DreamFusion} \cite{stable-dreamfusion} baseline. We first start by defining three python lists (aka. Prompt Builder Ingredients), viz. \texttt{objects}, \texttt{modifiers}, and \texttt{colors}. The \texttt{objects} list is set to verbose names of the categories from the Co3Dv2 \cite{reizenstein21common} which we used in our experiments. \cref{tab:prompt-ingredients} describes the values for the ingredient lists in full. Then we generate a shuffled list of all prompts by taking a full outer-product of the ingredients and ensuring correct grammar.  
% using the \texttt{get\_all\_prompts} function as provided in the code listing in \cref{fig:prompt-building-code}. 
Some of the generated final prompts are given in the \cref{tab:sample_prompts}.

% \begin{code}[The code snippet used to populate the prompts used to distill 3D radiance fields using the stable-dreamfusion \cite{stable-dreamfusion} implementation. Please refer the \cref{tab:prompt_ingredients} for the values of \texttt{modifiers}, \texttt{colors}, and \texttt{objects}. \label{fig:prompt-building-code}]
% def a_or_an(char: str) -> str:
%     return "an" if char in "aeiou" else "a"

% def get_all_prompts(modifiers: List[str], colors: List[str], objects: List[str]) -> List[str]:
%     all_prompts = []
%     for modifier in [""] + modifiers:
%         for color in [""] + colors:
%             for obj in objects:
%                 if modifier:
%                     prompt = f"{a_or_an(modifier[0])} {modifier}"
%                     if prompt.endswith("of"):
%                         # an additional "a/an" is needed for modifiers ending with "of"
%                         # for instance "a dslr photo of a green apple"
%                         if color:
%                             prompt += f"{a_or_an(color[0])} {color}"
%                         else:
%                             prompt += f" {a_or_an(obj[0])}"
%                 else:
%                     if color:
%                         prompt = f"{a_or_an(color[0])} {color}"
%                     else:
%                         prompt = a_or_an(obj[0])
%                 prompt += f" {obj}"
%                 all_prompts.append(prompt)
%     random.shuffle(all_prompts)
%     return all_prompts
% \end{code}

\begin{table*}
\centering
\caption{The values of the builder ingredients \texttt{objects}, \texttt{modifiers}, and \texttt{colors} used for generating the prompts for stable-dreamfusion \cite{stable-dreamfusion}. \label{tab:prompt-ingredients}}
\begin{tabular}{|l|p{0.7\linewidth}|}
\hline
\textbf{Prompt Builder Ingredient} & \textbf{Values used}  \\
\hline
\texttt{objects}   &  ``apple", ``water hydrant", ``teddy bear", ``donut" \\
\hline
\texttt{modifiers} & ``unreal render of", ``zoomed out unreal render of", ``wide angle zoomed out unreal render of", ``dslr photo of", ``zoomed out dslr photo of", ``wide angle zoomed out dslr photo of", ``plastic", ``metallic", ``wooden", ``furry" \\
\hline
\texttt{colors}    & ``red", ``green", ``blue", ``yellow",  ``orange", ``brown", ``pink", ``purple", ``cyan", ``magenta", ``sky blue", ``baby blue", ``crimson", ``lime", ``teal", ``violet", ``sea green", ``dusk", ``gold", ``silver" \\
\hline
\end{tabular}
\end{table*}

\begin{table}
\centering
\caption{A sampling of the prompts generated after running the prompt-building process. \label{tab:sample_prompts}}
\begin{tabular}{|p{1.0\linewidth}|}
\hline
\textbf{Sample prompts} \\
\hline
 ``\texttt{a plastic teddy bear}'', \\
 ``\texttt{a zoomed out unreal render of a water hydrant}'', \\
 ``\texttt{a wide angle zoomed out unreal render of a dusk donut}'', \\
 ``\texttt{a dslr photo of a water hydrant}'', \\
 ``\texttt{a plastic apple}'', \\
 ``\texttt{a sea green apple}'', \\
 ``\texttt{an unreal render of a red apple}'', \\
 ``\texttt{an unreal render of a silver donut}'', \\
 ``\texttt{a baby blue water hydrant}'', \\
 ``\texttt{a metallic donut}'' \\
\hline
\end{tabular}
\end{table}

% \section{Additional qualitative results}
% We provide a zip containing an  html-page that can be viewed \textit{locally} using any browser (we recommend firefox). The html shows supplementary videos of our results. In order to view the webpage, please unzip the zip file provided as a part of the supplementary material and open the \texttt{focussed\_results.html}.
